# Supplementary material for: DynamicKV: Task-Aware Adaptive KV Cache Compression for Long Context LLMs
Source: arXiv:2412.14838 source file (2025-05-27)
Supplement: Supplementary file 1 [file 07_appendix_all_models.tex]

\begin{figure}[htbp]
    \centering
    \begin{subfigure}[b]{0.45\textwidth}
        \includegraphics[width=\textwidth]{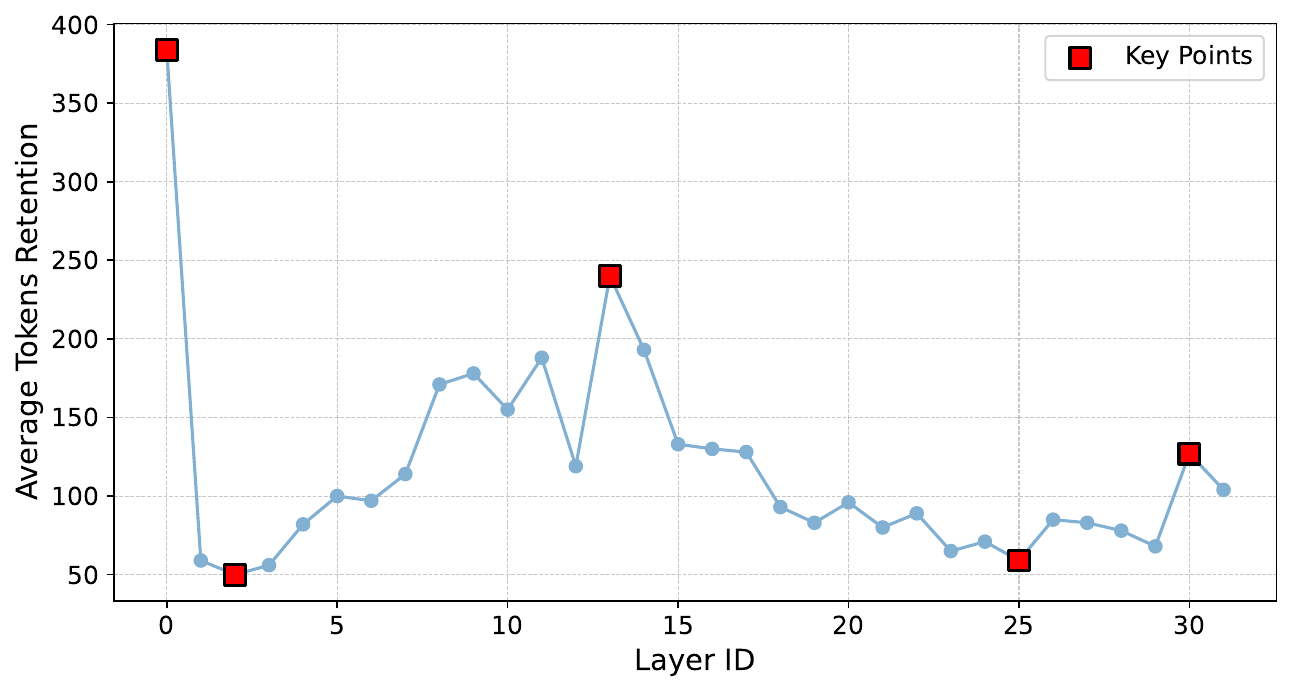}
        \caption{Llama-3-8B-Instruct}
    \end{subfigure}
    \hfill
    \begin{subfigure}[b]{0.45\textwidth}
        \includegraphics[width=\textwidth]{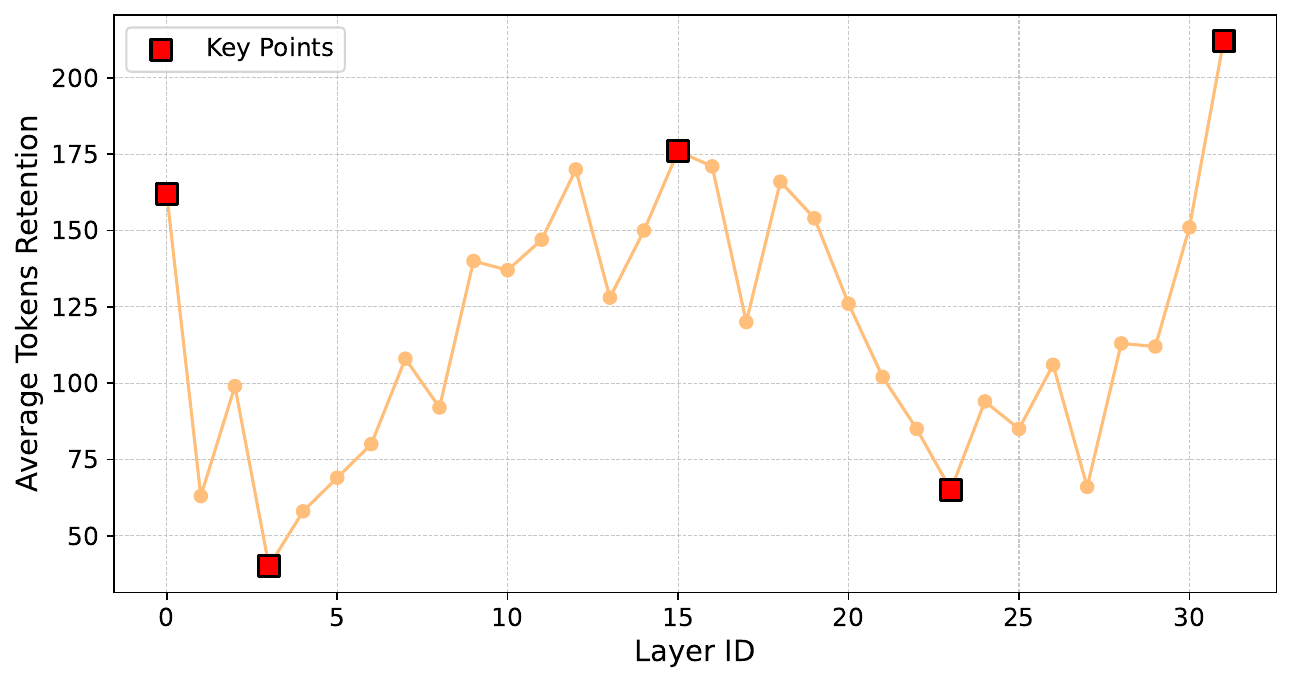}
        \caption{Mistral-7B-Instruct}
    \end{subfigure}
    % \hfill
    \vspace{1em} 
    \begin{subfigure}[b]{0.45\textwidth}
        \includegraphics[width=\textwidth]{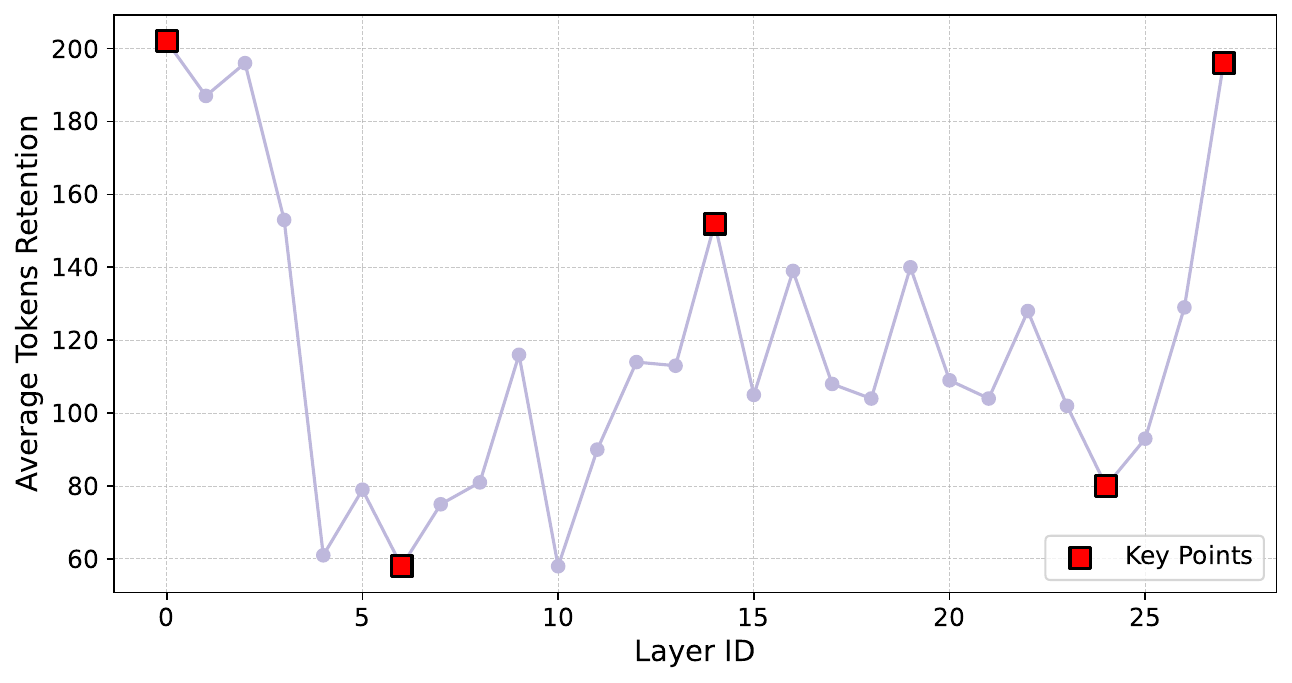}
        \caption{Qwen-2-7B-Instruct}
    \end{subfigure}
    \hfill
    \begin{subfigure}[b]{0.45\textwidth}
        \includegraphics[width=\textwidth]{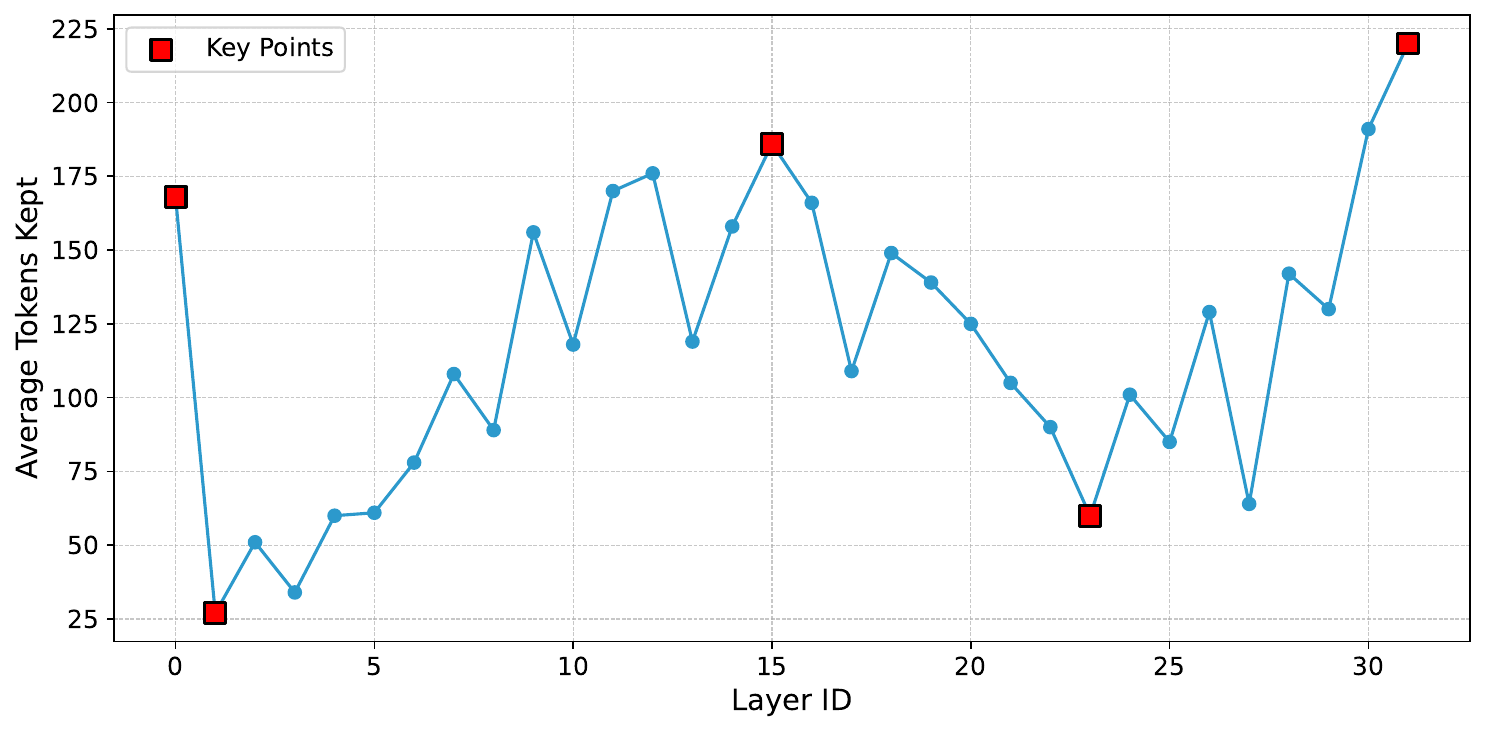}
        \caption{InternLM-2.5-7B-Chat-1M}
    \end{subfigure}
    \caption{Average KV cache per layer for different models on the LongBench dataset.}
    \label{fig:longbench_all_models}
\end{figure}
